# Supplementary material for: Enhancing ML-Based DoS Attack Detection Through Combinatorial Fusion Analysis
Source: arXiv:2312.00006 source file (2023-10-02)
Supplement: Supplementary file 1 [file appendix.tex]

\begin{figure*}[htbp]
    \centering
    \includegraphics[height=15cm, width=14cm]{figures/Http_layer_Data_Capture_Algorithm.drawio.pdf}
    \caption{Flow chart for our HTTP layer data capture process.}
    \label{fig:http-capture}
\end{figure*}
